# Supplementary material for: Fast and Versatile RNA Design via Motif-level Divide-and-Conquer and Structure-level Rival Search
Source: arXiv:2603.02283 source file (2026-03-02)
Supplement: Supplementary file 1 [file appendix.tex]

% !TEX root = main.tex

%\appendix
\begin{appendices}
%\onecolumn

%{\centering \large Supplementary Information}
%\author{Ning Dai\inst{1} \and
%Milan Gautam\inst{1} \and
%Tianshuo Zhou\inst{1} \and
%David H. Mathews\inst{3, 4, 5}  \and
%Liang Huang\inst{1,2} }

\setcounter{figure}{0}
 % spacing

\setcounter{table}{0}

\setcounter{section}{0}

\setcounter{footnote}{0}

%\authorrunning{N.~Dai, M.~Gautam et al.}
% First names are abbreviated in the running head.
% If there are more than two authors, 'et al.' is used.
%
%\institute{$^1$ School of EECS and
%$^2$ Dept.~of Biochemistry \& Biophysics, Oregon State University, Corvallis OR 97330, USA \\
%$^3$ Dept.~of Biochemistry \& Biophysics, 
%%University of Rochester Medical Center, Rochester, NY 14642, USA\\
%%\and
%$^4$ Center for RNA Biology, 
%%University of Rochester Medical Center, Rochester, NY 14642, USA\\
%and $^5$ Dept.~of Biostatistics \& Computational Biology, University of Rochester Medical Center, Rochester, NY 14642, USA
%}
%%
%\maketitle
%\input{supp}

\begin{figure*}%[h]
\centering
  \hspace{-0.2cm}
  \begin{tabular}{ccc}
    \includegraphics[width=0.33\linewidth]{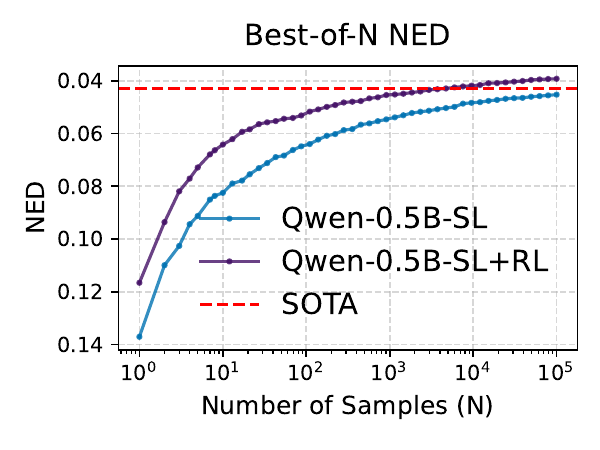}
    &
    \includegraphics[width=0.33\linewidth]{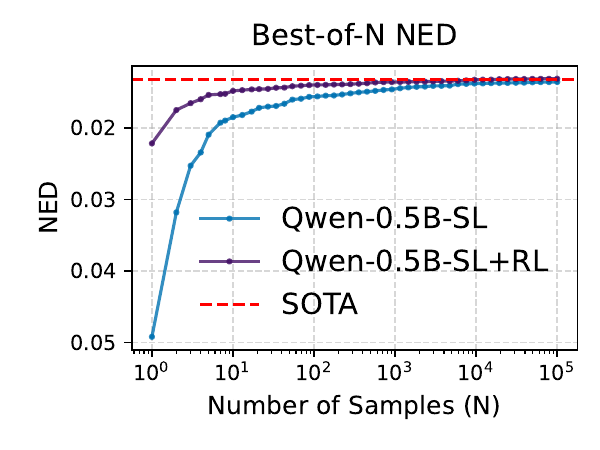}
    &
    \includegraphics[width=0.33\linewidth]{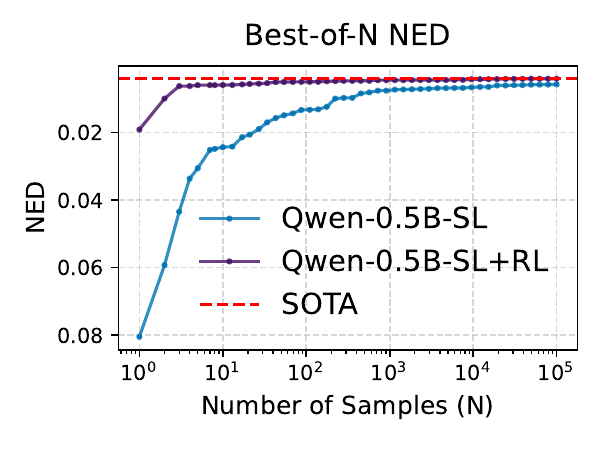}
    \\[-0.2cm]
    (a) Eterna100 & (b) RNAsolo100 & (c) Rfam-Taneda-27
  \end{tabular}
  \vspace{-0.2cm}
\caption{Best-of-$N$ curves for SL and SL+RL models in terms of normalized ensemble defect (NED) on three data sets. Our SL+RL model 
outperforms (or ties with) SOTA on NED on all test sets. See Fig.~\ref{fig:SL+RL} in the main text for the corresponding Best-of-$N$ curves on Boltzmann probability.}
\label{fig:SI-SL+RL}
\end{figure*}

\begin{table}[h!]
\centering
\setlength{\arrayrulewidth}{1pt}

\begin{tabular}{l|cc}
\hline
Method 
  & \multicolumn{2}{c}{\# of MFE/uMFE ($\uparrow$)} \\
\cline{2-3}
  & Eterna100
  & Rfam-Taneda-27 \\
\hline
Eastman \emph{et al.} (\cite{eastman+:2018})
  & 60 / 42
  & -- / -- \\
LEARNA (\cite{runge+:2019})
  & 67 / --
  & 23 / -- \\
Meta-LEARNA (\cite{runge+:2019})
  & 68 / --
  & {\bf 24} / -- \\
\hline
Ours (SL+RL)
  & \textbf{75 / 73}
  & {\bf 24} / 24 \\

\hline
\end{tabular}

\caption{Comparison of RL methods on Eterna100 and Rfam-Taneda-27. The baselines' numbers are taken from those papers and they only reported MFE metrics.
Our work substantially outperforms them on Eterna100.}
\label{tab:SI-RL}
\end{table}

\end{appendices}

% \caption{compare with RL baselines}
% \end{table}

% \begin{figure}[t]
%   \centering
%   \hspace{-0.2cm}
%   \begin{tabular}{ccc}
%     \includegraphics[width=0.33\linewidth]{figs/best_of_N_ensemble_defect_eterna.pdf}
%     &
%     \includegraphics[width=0.33\linewidth]{figs/best_of_N_ensemble_defect_RNAsolo.pdf}
%     &
%     \includegraphics[width=0.33\linewidth]{figs/best_of_N_ensemble_defect_rfam.pdf}
%     \\[-0.2cm]
%     (a) Eterna100 & (b) RNAsolo100 & (c) Rfam-Taneda-27
%   \end{tabular}
%   \vspace{-0.2cm}
% \caption{Best-of-$N$ curves for SL and SL+RL models in terms of normalized ensemble defect (NED) on three data sets. Our SL+RL model 
% outperforms (or ties with) SOTA on NED on all test sets. See Fig.~\ref{fig:SL+RL} in the main text for the corresponding Best-of-$N$ curves on Boltzmann probability.}
% \end{figure}
